# Supplementary material for: The many reasons that the rotation curves of low-mass galaxies can fail as tracers of their matter distributions
Source: arXiv:2301.05242 ancillary file (2023-06-29)

8.94 Gyr

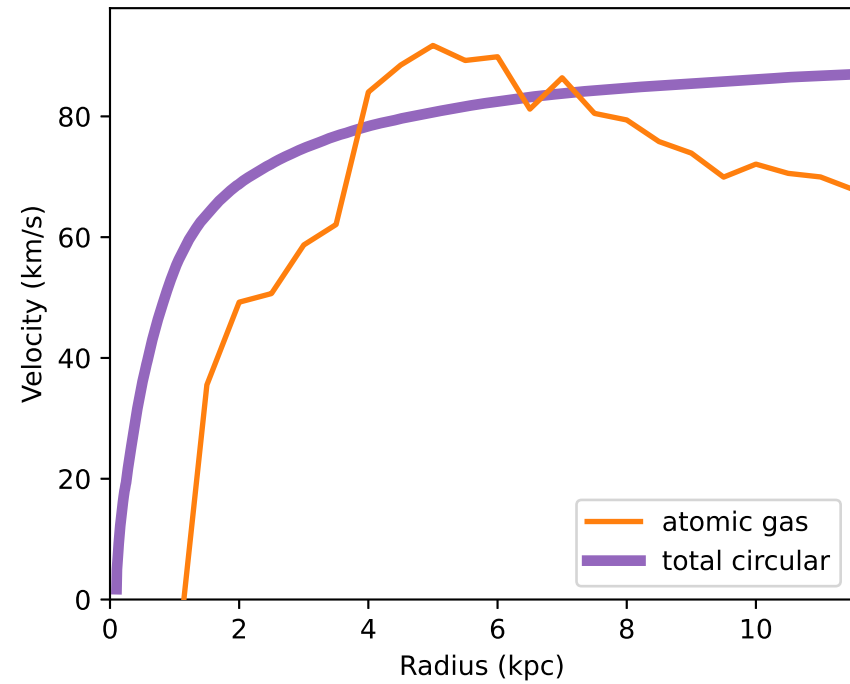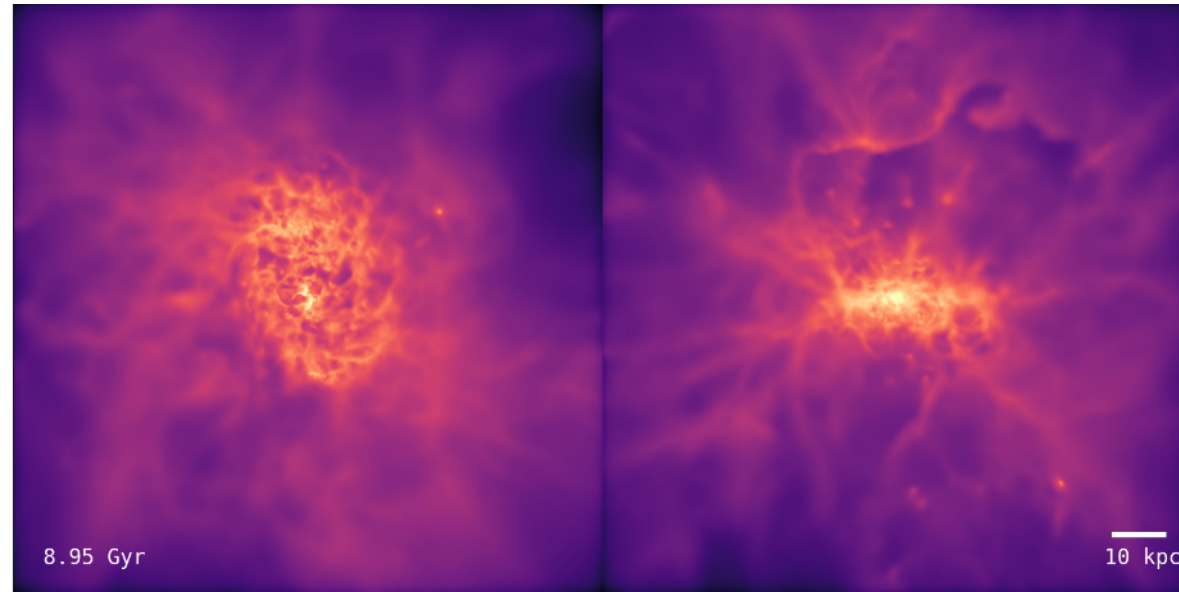

9.21 Gyr

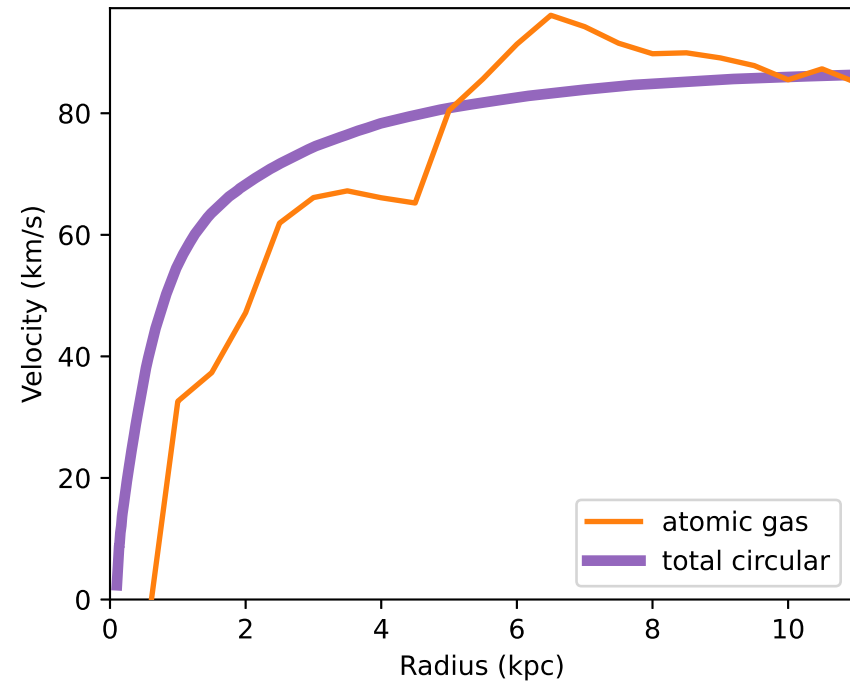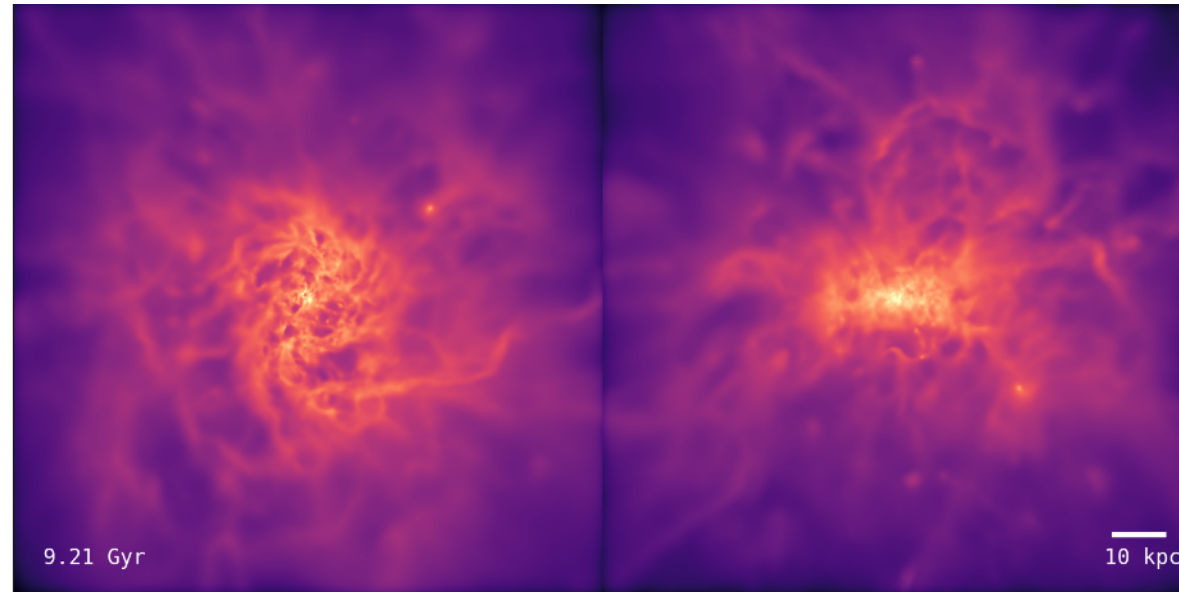

9.48 Gyr

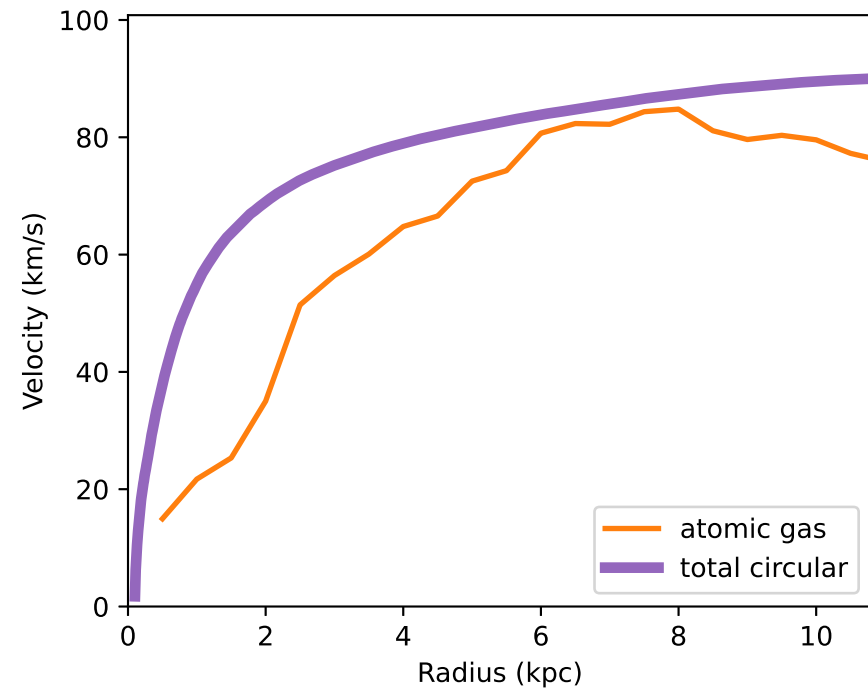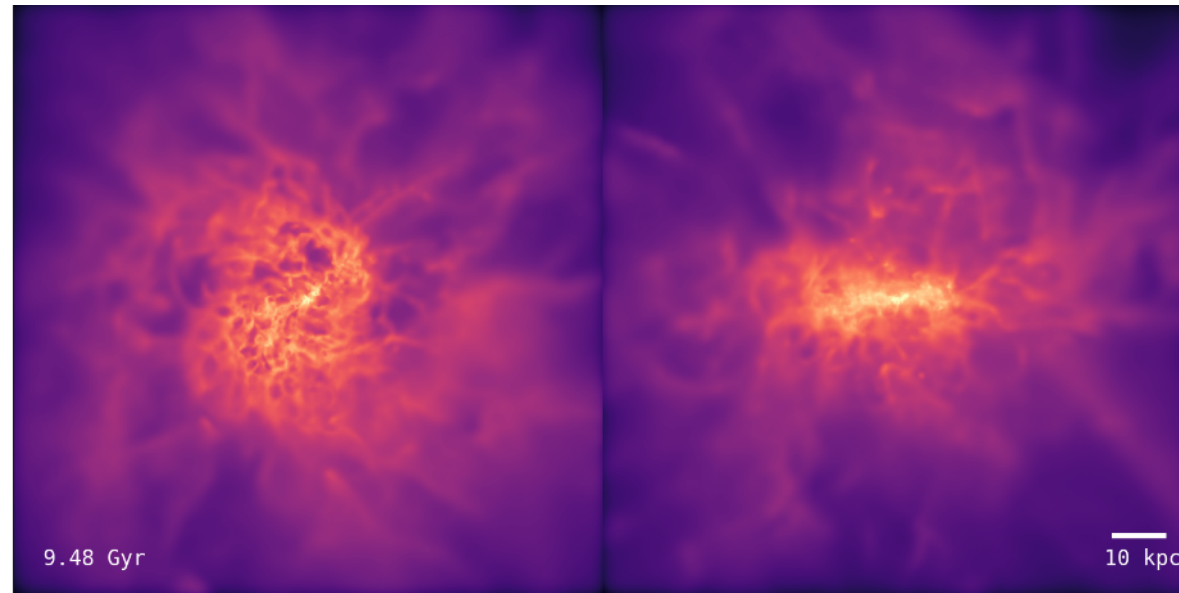

9.76 Gyr

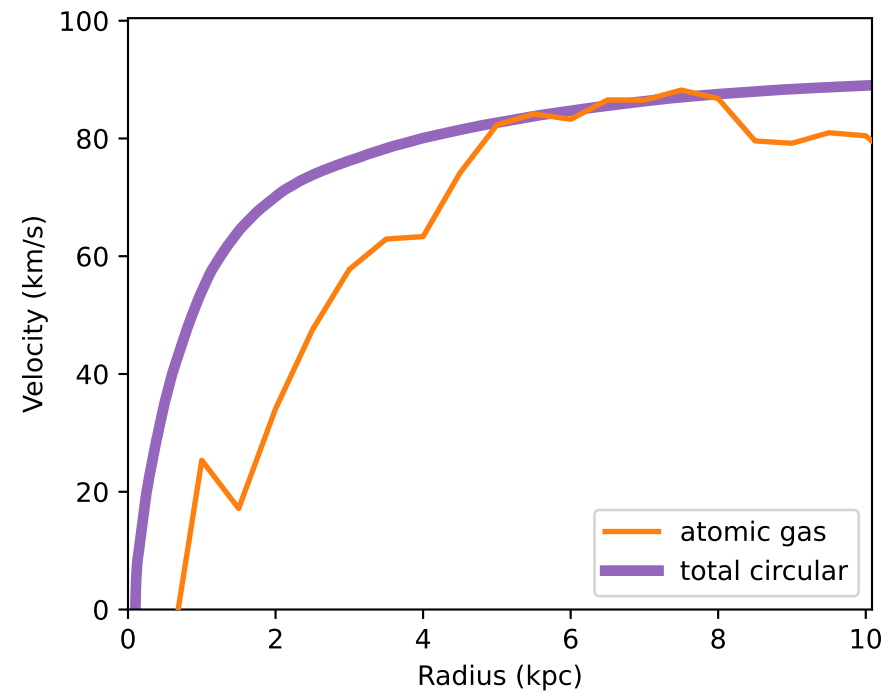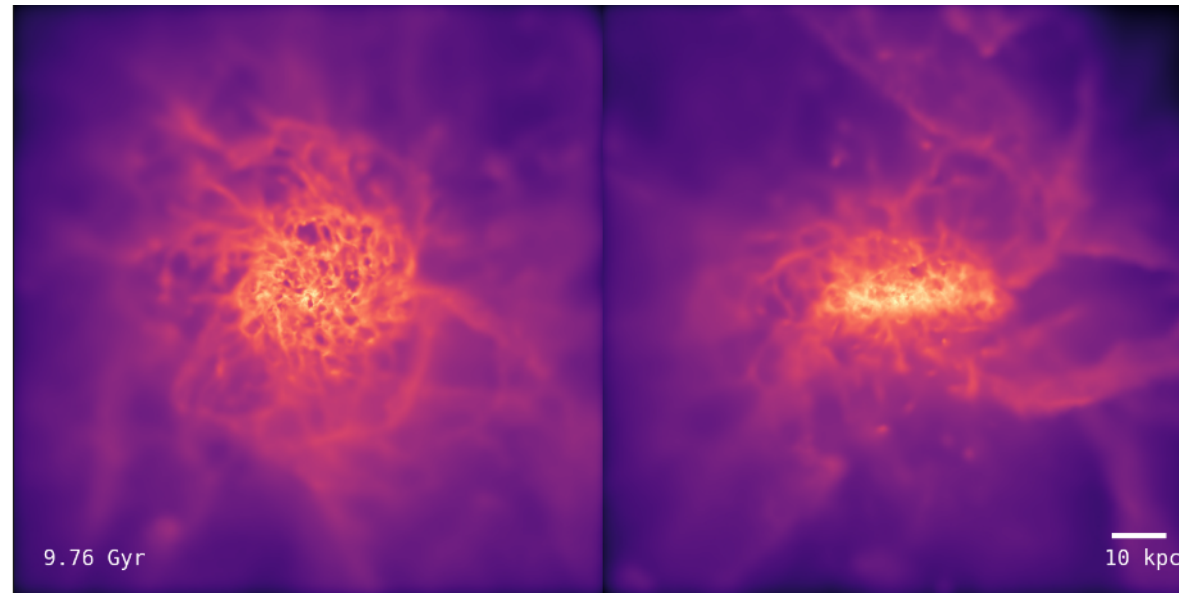

10.04 Gyr

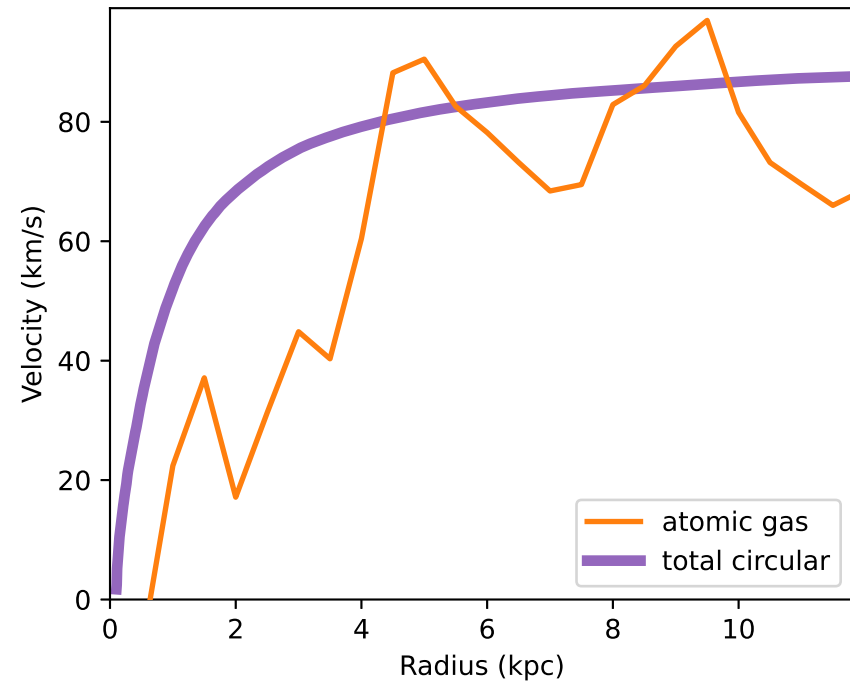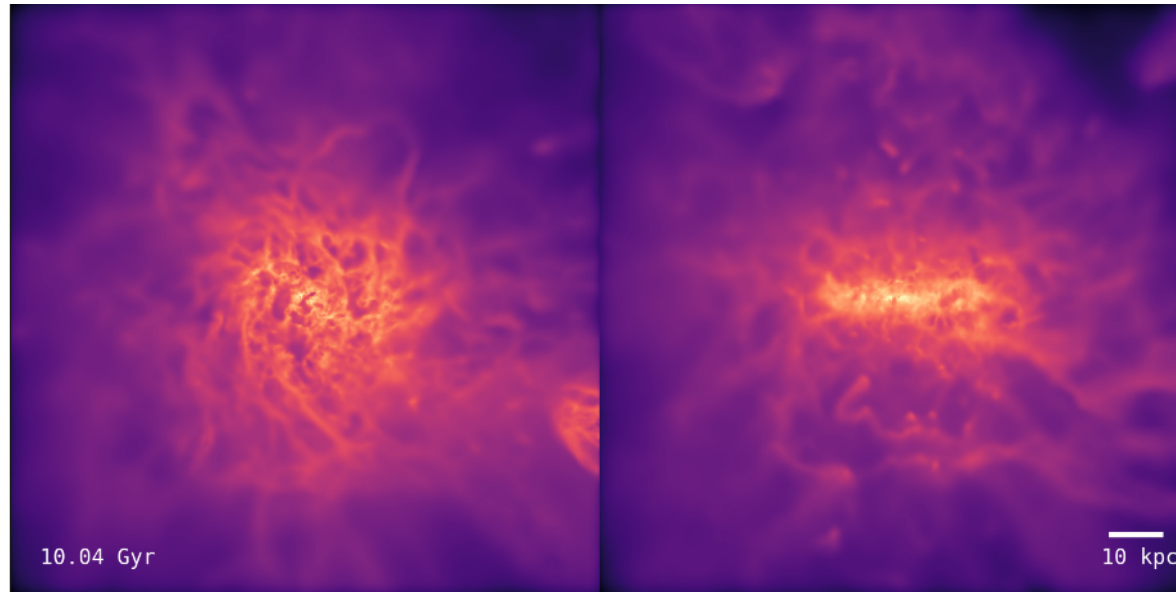

10.32 Gyr

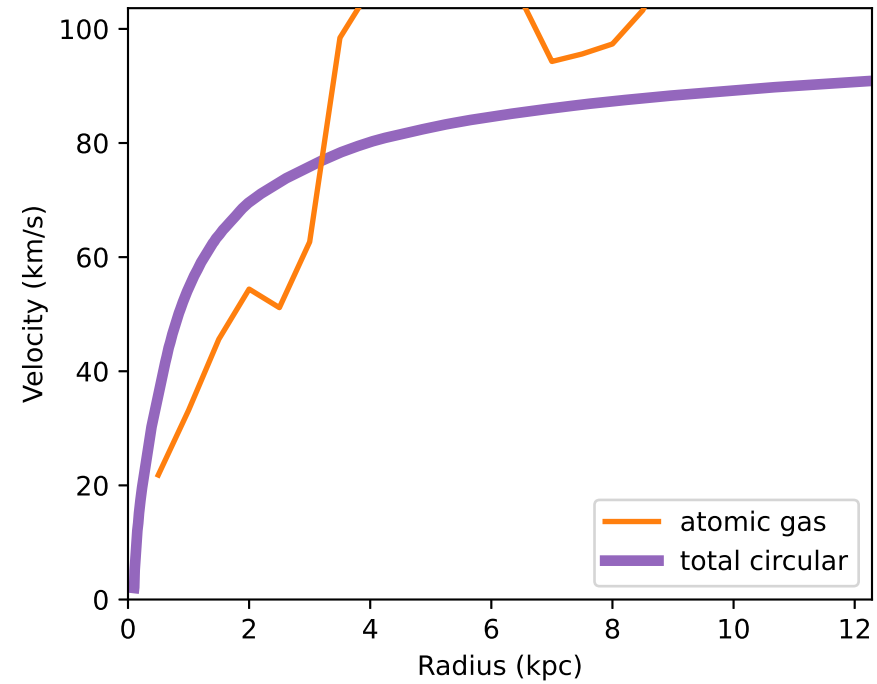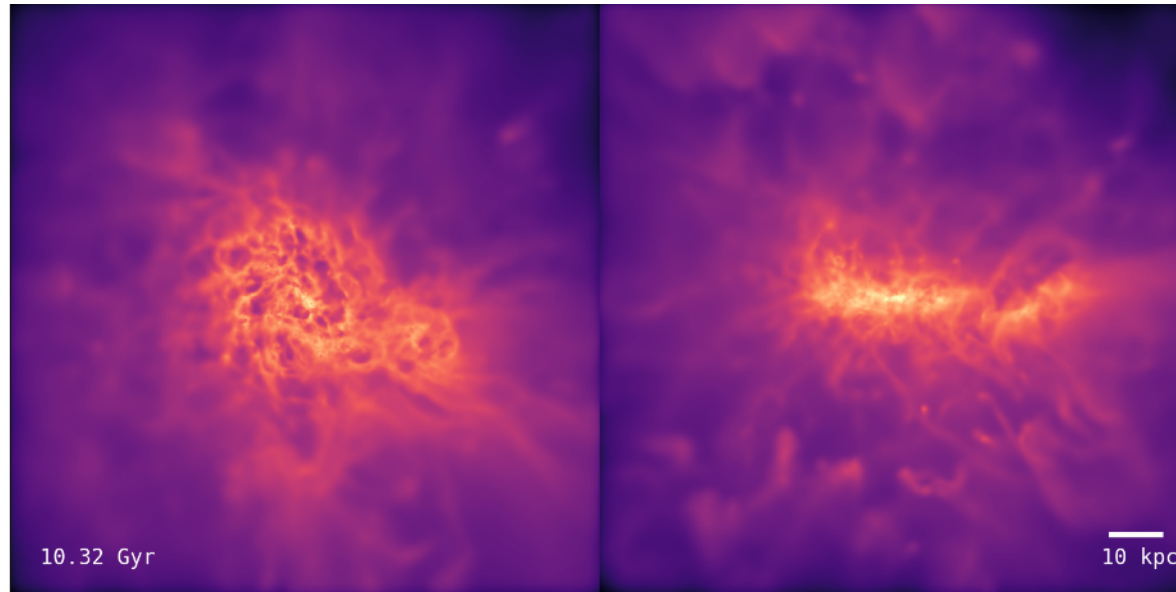

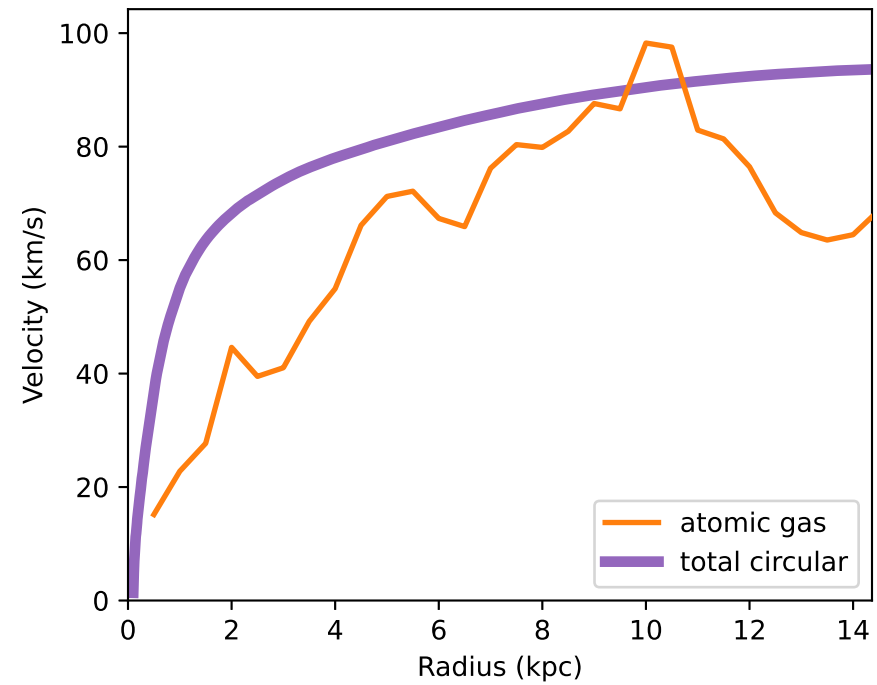

10.62 Gyr

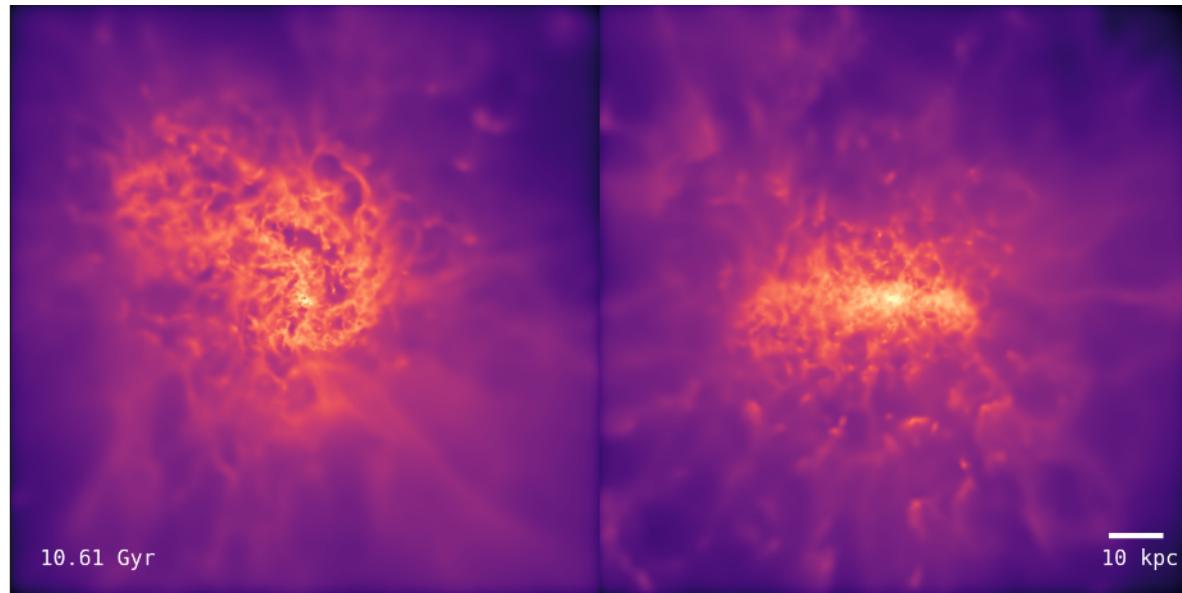

10.91 Gyr

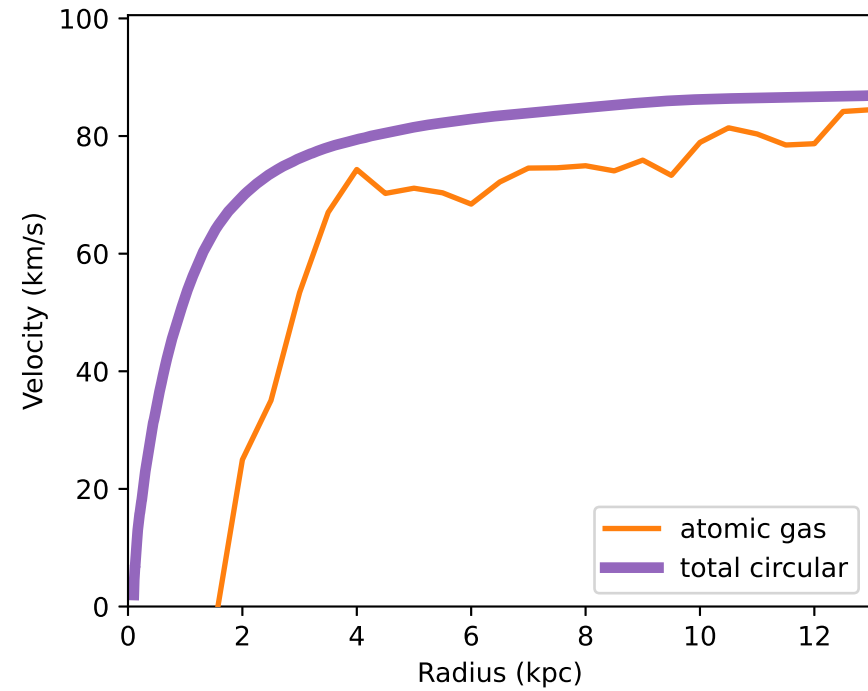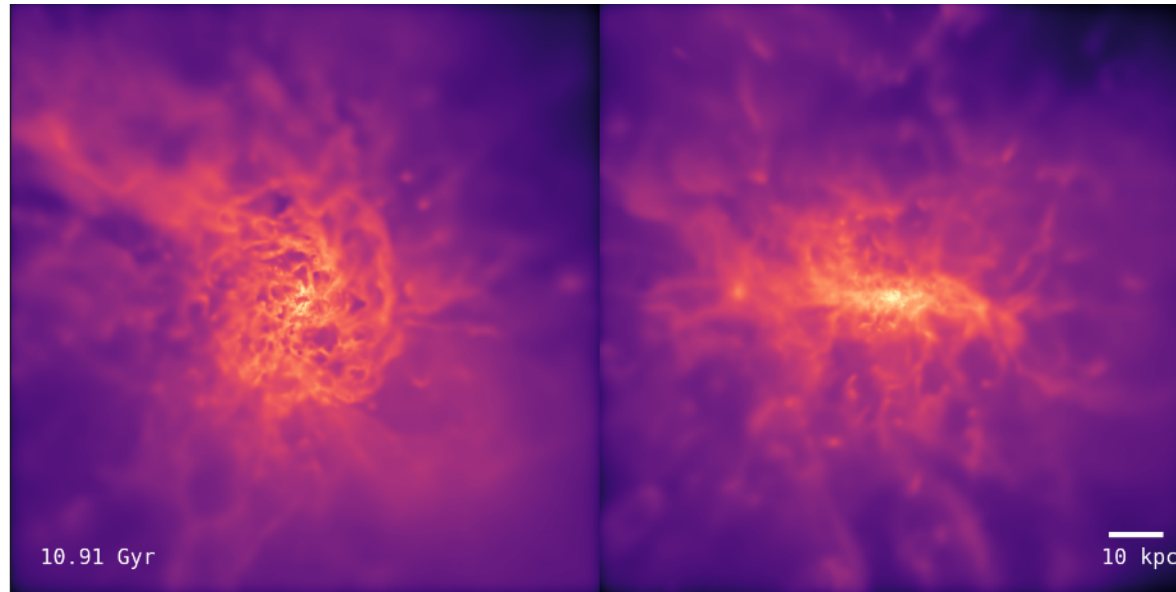



11.21 Gyr

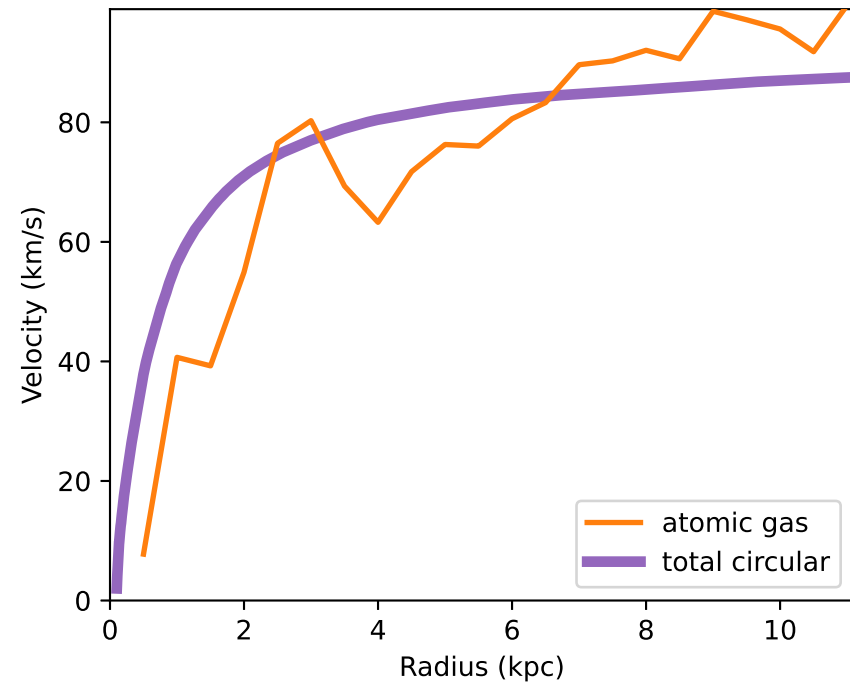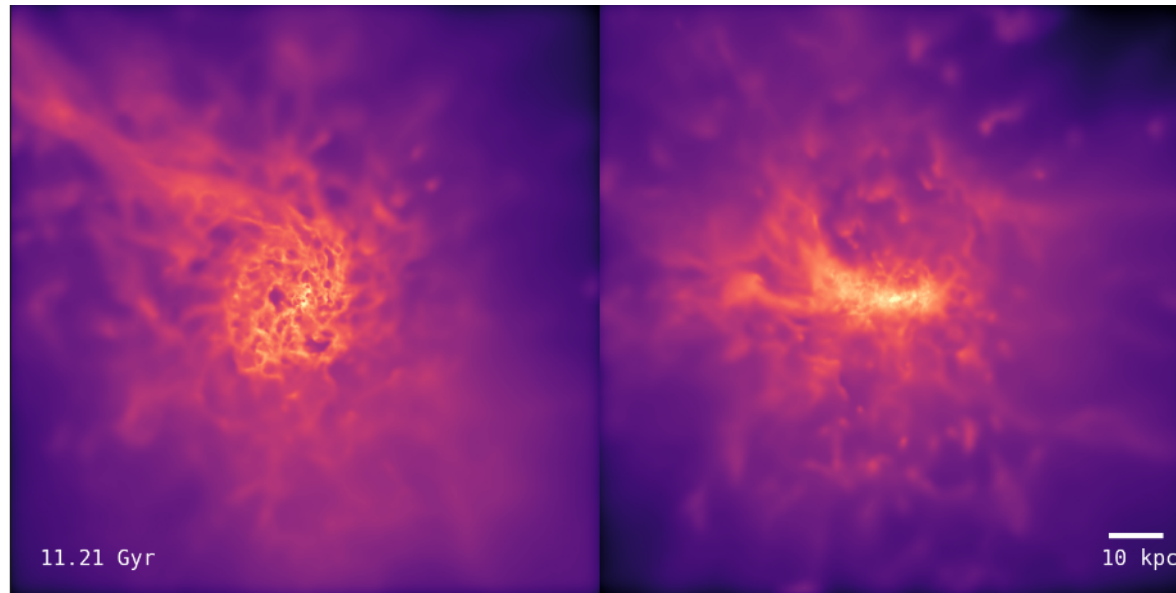

11.52 Gyr

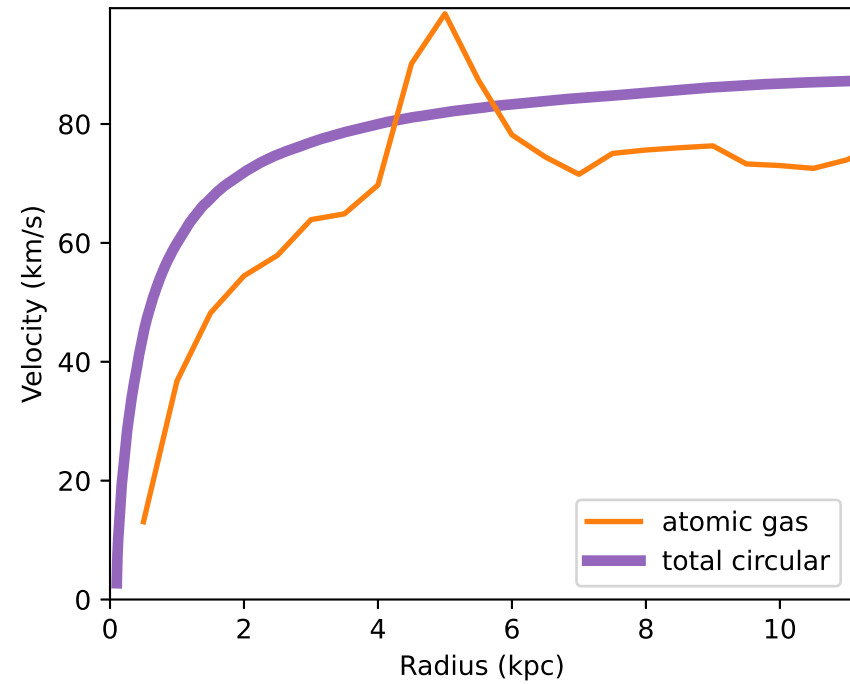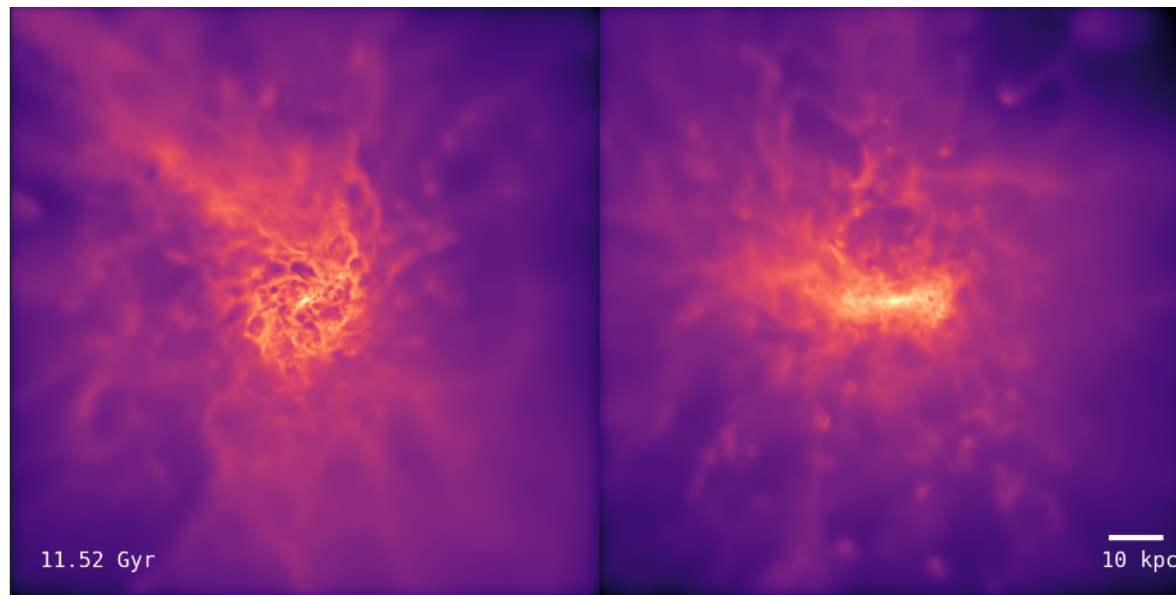

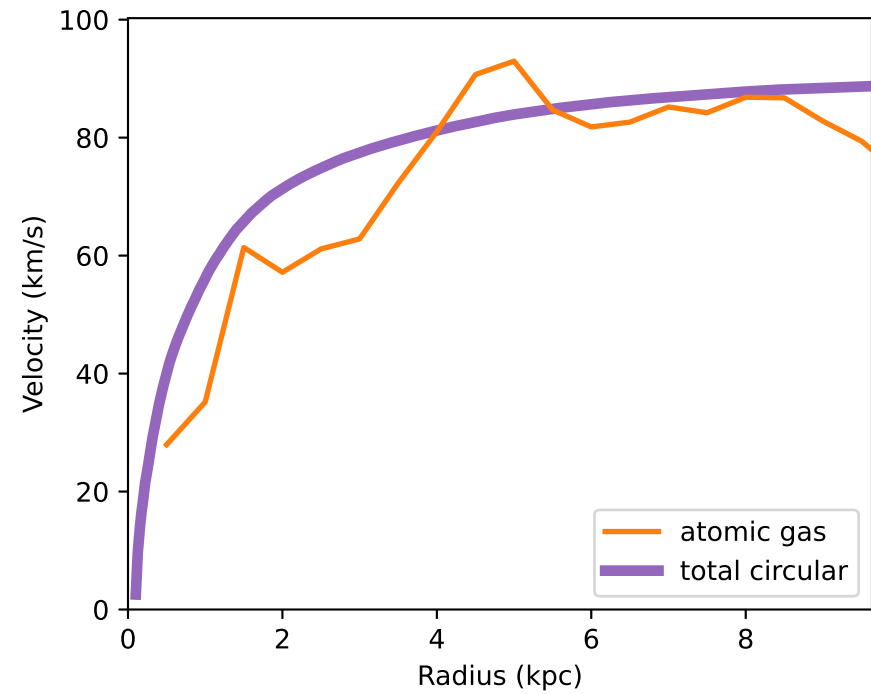

11.83 Gyr

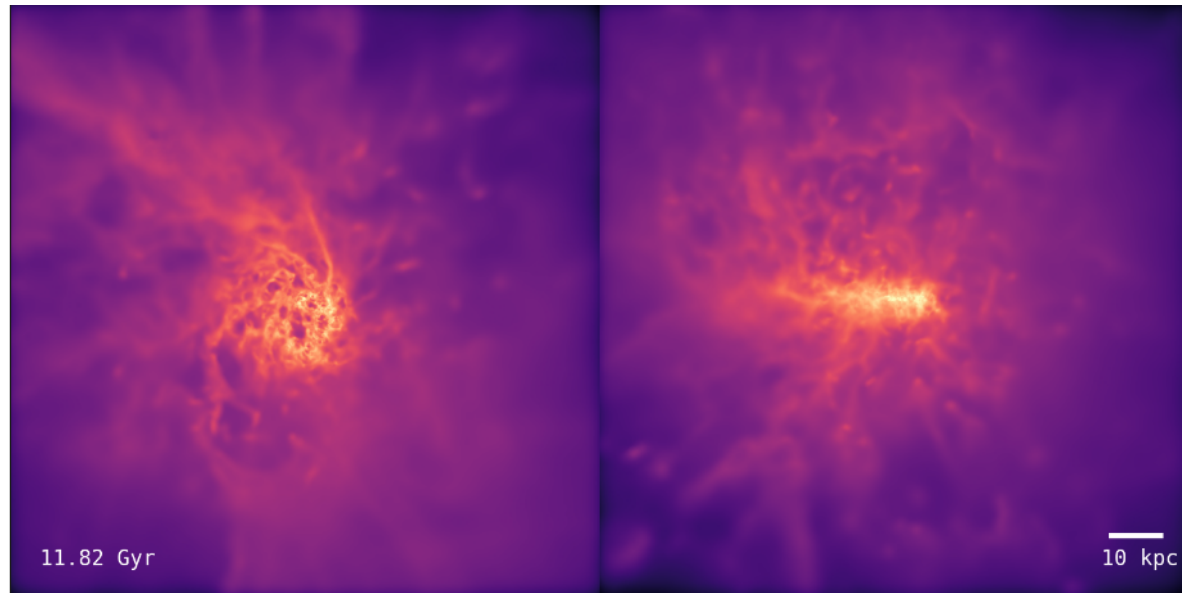

12.14 Gyr

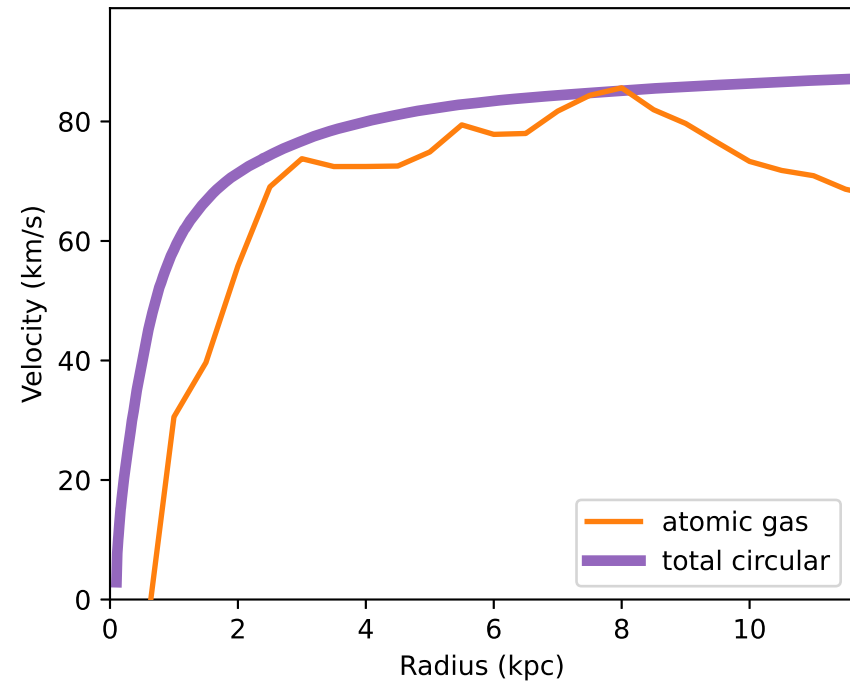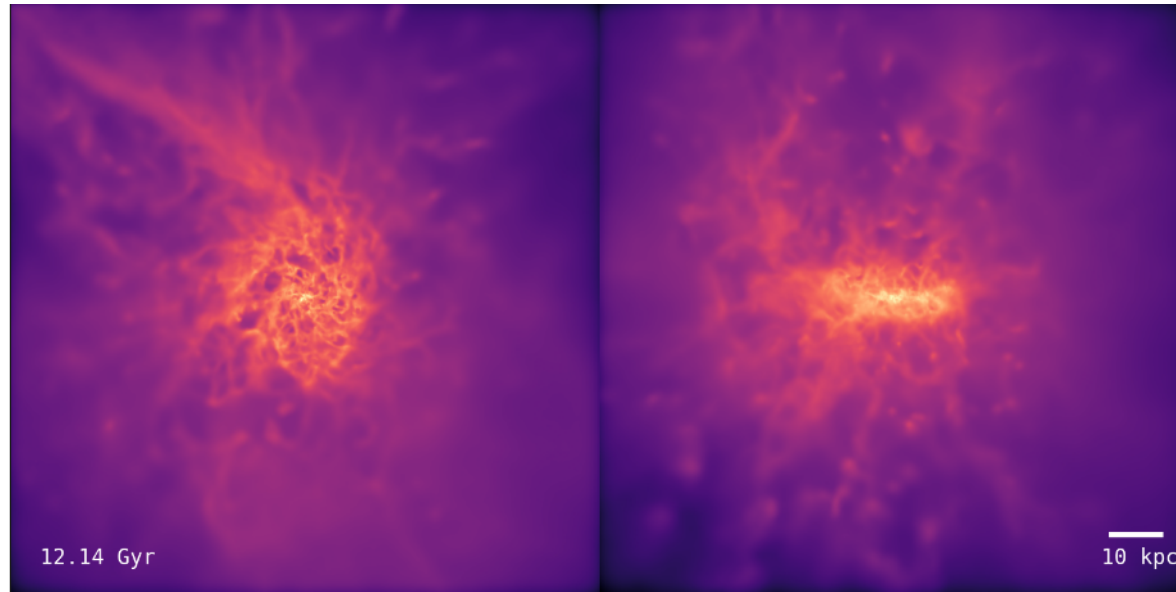

12.46 Gyr

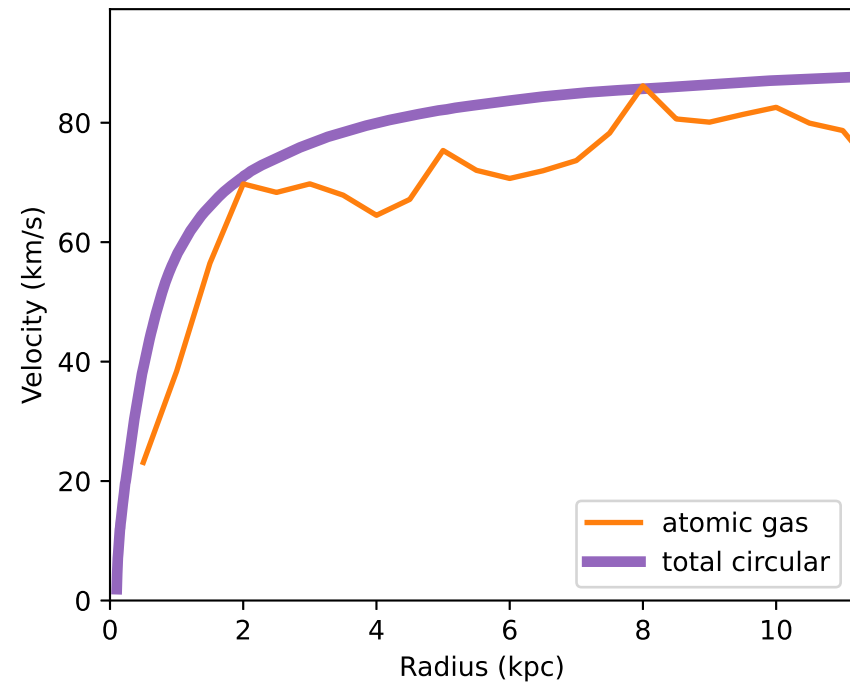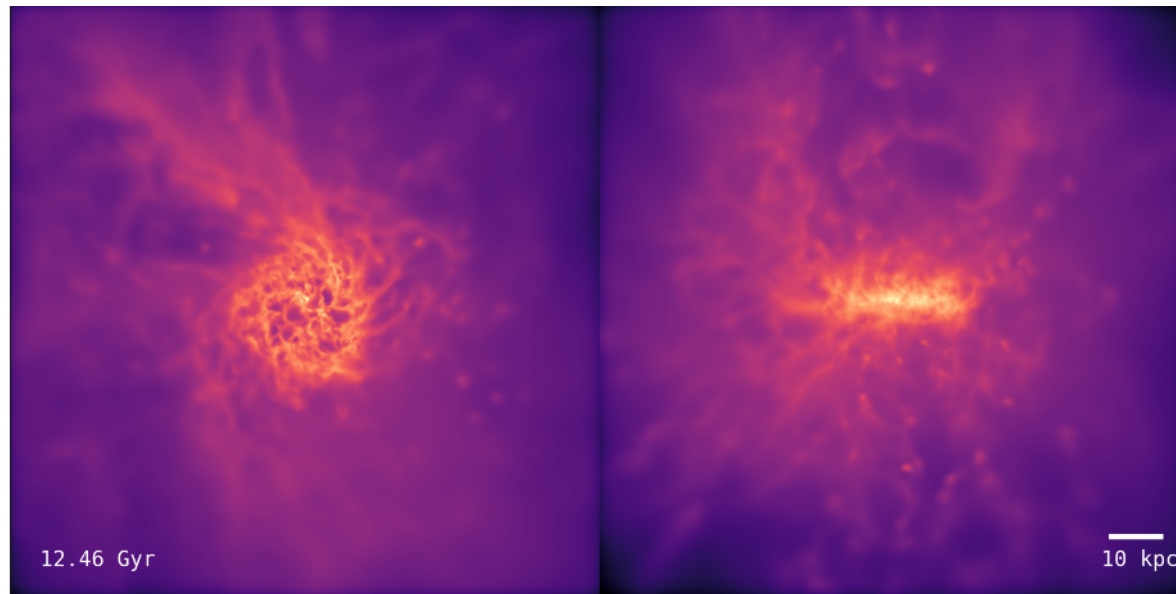

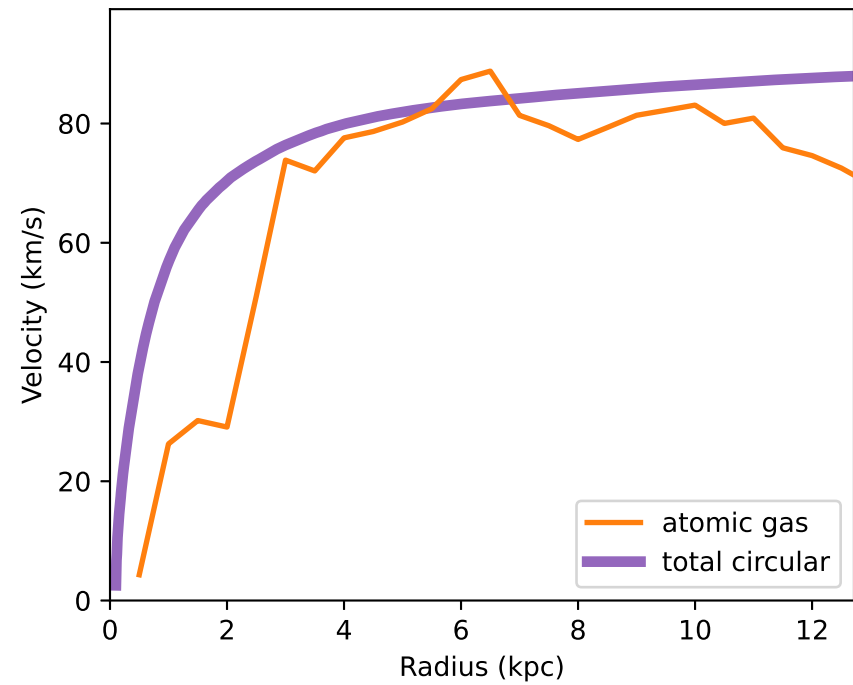

12.78 Gyr

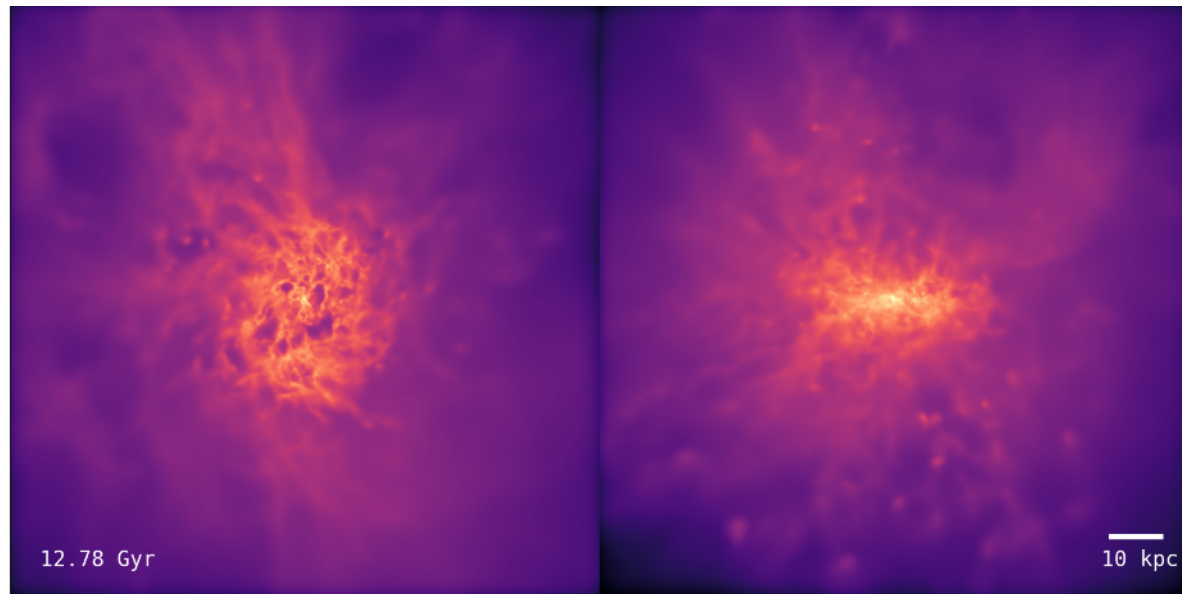

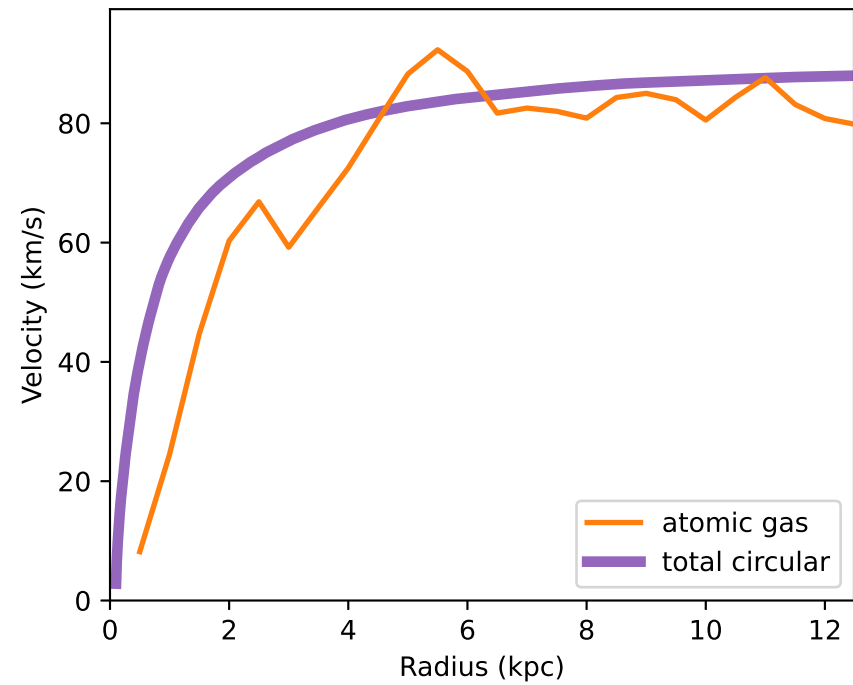

13.10 Gyr

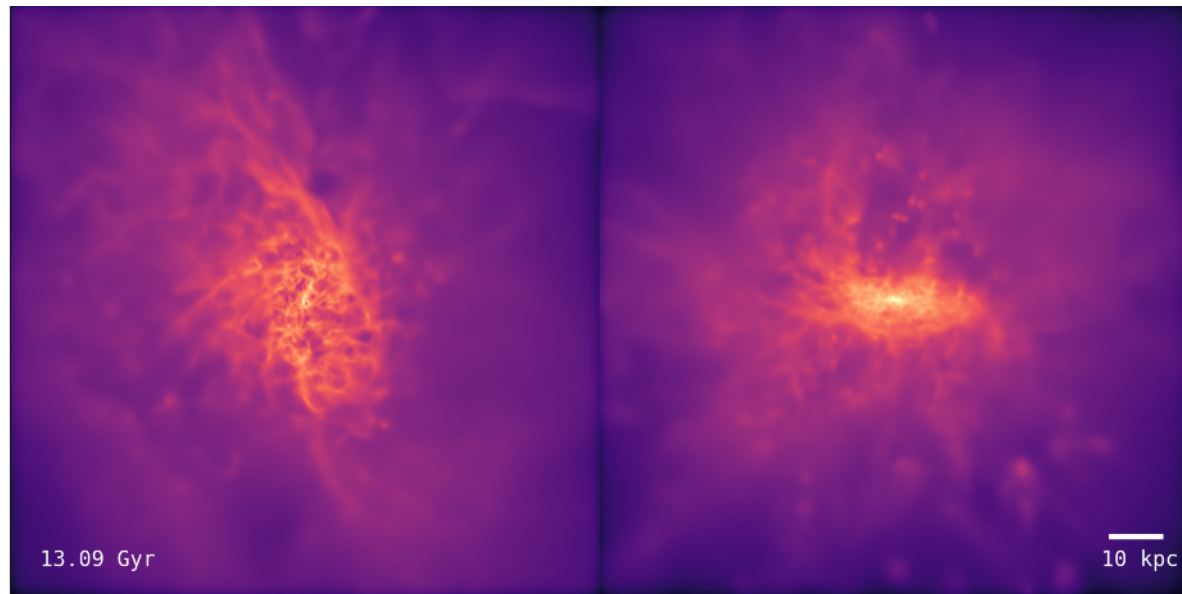

13.43 Gyr

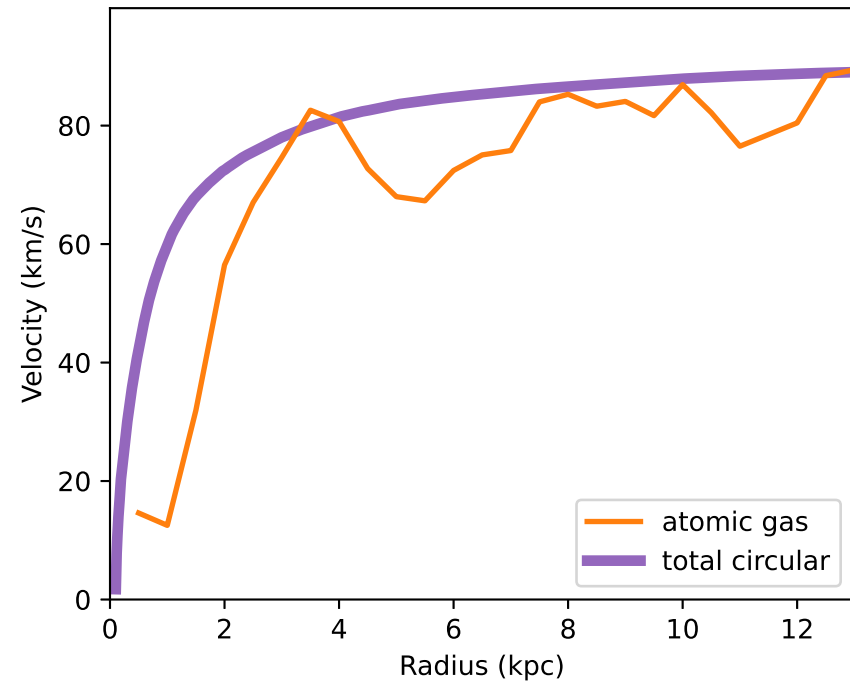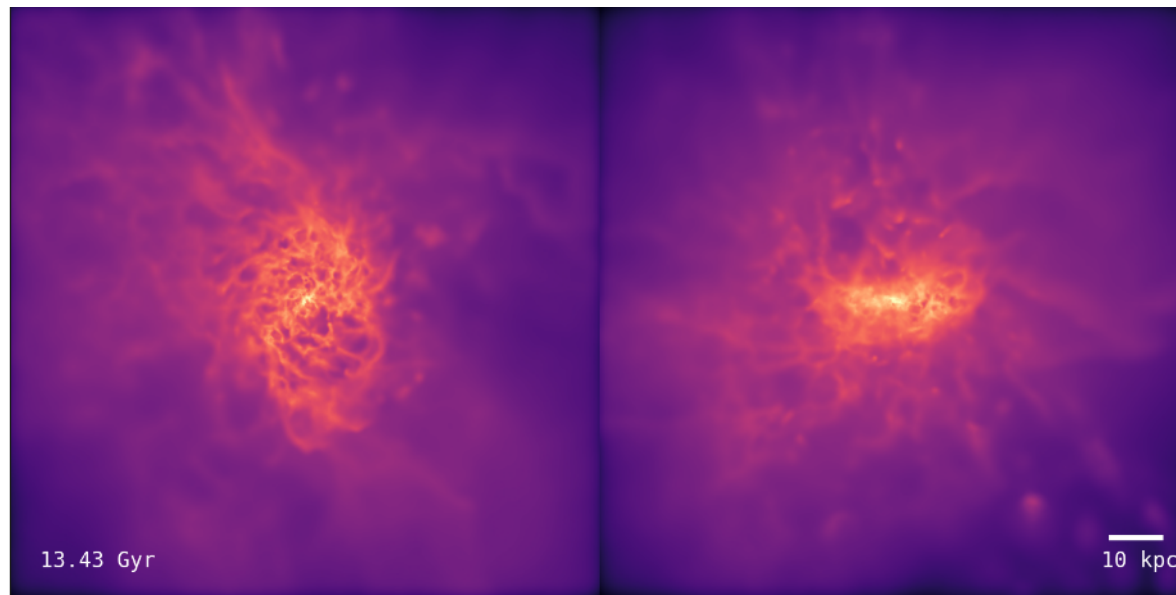



13.76 Gyr

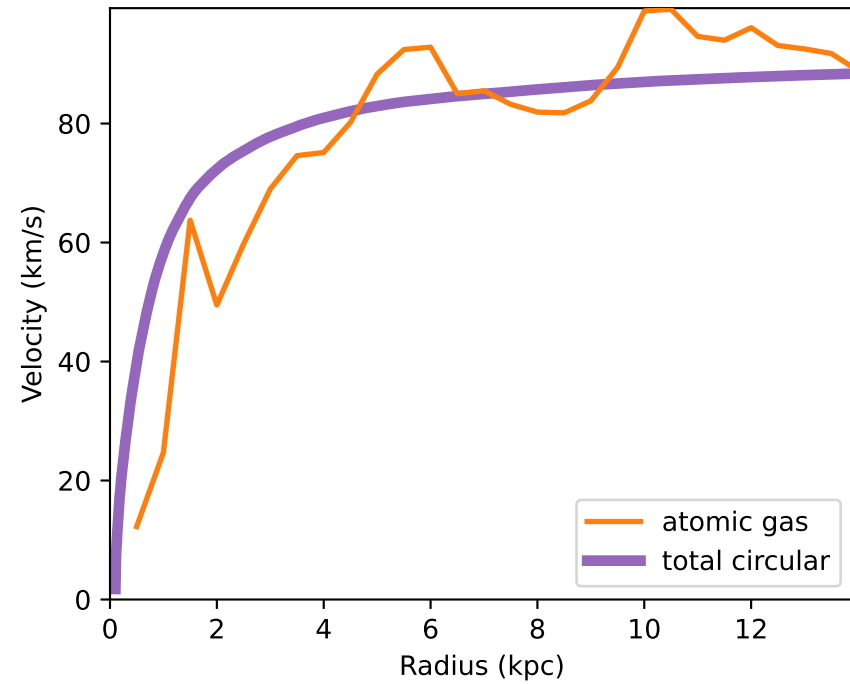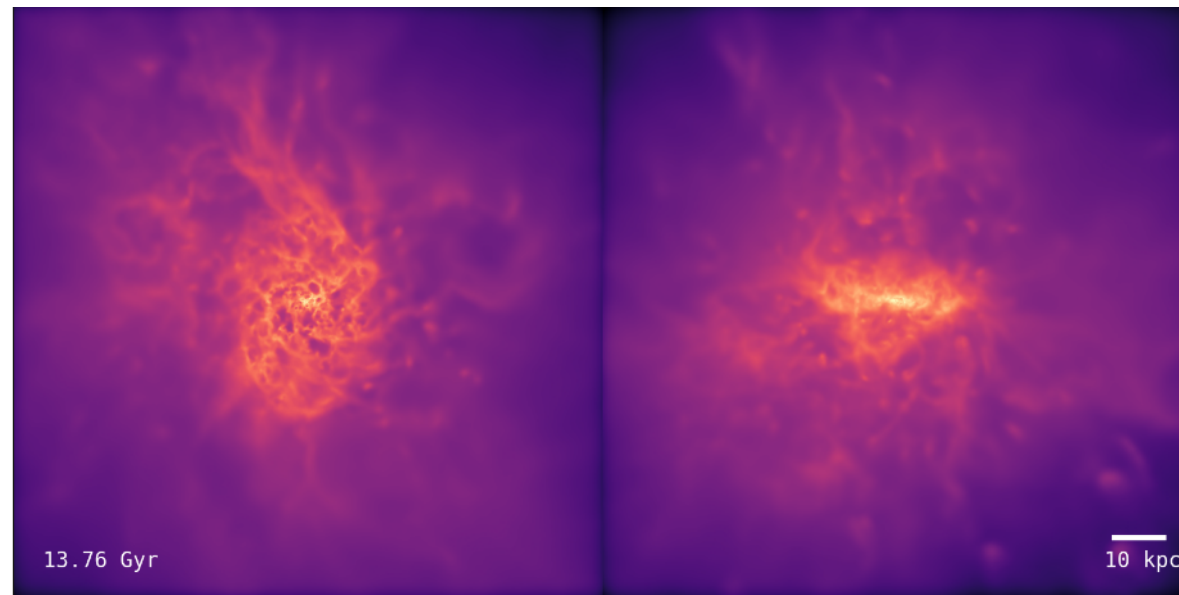

Supplement: Supplementary file 1 [file AP-L1-V6-5-0-rotation-curves.pdf]
